# Supplementary material for: START: Spatial and Textual Learning for Chart Understanding
Source: arXiv:2512.07186 source file (2025-12-08)
Supplement: Supplementary file 1 [file supplement.tex]

% WACV 2026 Paper Template
% based on the ICCV 2025 template (https://media.eventhosts.cc/Conferences/ICCV2025/ICCV2025-Author-Kit-Feb.zip) with
% WACV-specific details (e.g., 2 tracks) from the WACV 2025 template (https://www.dropbox.com/scl/fi/su44zgdhrzik26p2xu37k/WACV-2025-Author-Kit-Template.zip?rlkey=5qcfimjhxnmx3wlyk7yhk8wg7&dl=0)

\documentclass[10pt,twocolumn,letterpaper]{article}

%%%%%%%%% PAPER TYPE  - PLEASE UPDATE FOR FINAL VERSION
\usepackage[review,algorithms]{wacv}      % To produce the REVIEW version for the algorithms track
%\usepackage[review,applications]{wacv}      % To produce the REVIEW version for the applications track
%\usepackage{wacv}              % To produce the CAMERA-READY version
% \usepackage[pagenumbers]{wacv} % To force page numbers, e.g. for an arXiv version

% Import additional packages in the preamble file, before hyperref
\input{preamble}
\usepackage{multirow}
\usepackage{mathtools}
\usepackage{minted}

% Optional: Customize the appearance. 
% This sets a light gray background for all minted environments.
\setminted{
    bgcolor=gray!10, % Light gray background (10% gray)
    fontsize=\small, % Use a smaller font size
    linenos,         % Add line numbers
    frame=lines,     % Add a frame around the code
    framesep=2mm,
    breaklines       % Automatically break long lines
}
% It is strongly recommended to use hyperref, especially for the review version.
% hyperref with option pagebackref eases the reviewers' job.
% Please disable hyperref *only* if you encounter grave issues, 
% e.g. with the file validation for the camera-ready version.
%
% If you comment hyperref and then uncomment it, you should delete *.aux before re-running LaTeX.
% (Or just hit 'q' on the first LaTeX run, let it finish, and you should be clear).
\definecolor{wacvblue}{rgb}{0.21,0.49,0.74}
\usepackage[pagebackref,breaklinks,colorlinks,allcolors=wacvblue]{hyperref}

%%%%%%%%% PAPER ID  - PLEASE UPDATE
 % *** Enter the WACV Paper ID here

%%%%%%%%% TITLE - PLEASE UPDATE
\title{START: \underline{S}patial and \underline{T}extual Learning for Ch\underline{art} Understanding \
(Supplementary Material)}

% %%%%%%%%% AUTHORS 

%\vspace{-0.5cm}
% \author{Zhuoming Liu\textsuperscript{1\thanks{Work done during internship at Amazon AGI.}}, Xiaofeng Gao\textsuperscript{2}, Feiyang Niu\textsuperscript{2}, Qiaozi Gao\textsuperscript{2}, Liu Liu\textsuperscript{3}, Yin Li\textsuperscript{1}, Robinson Piramuthu\textsuperscript{2}\\ 
% {\textsuperscript{1}University of Wisconsin-Madison \ \ 
% \textsuperscript{2}Amazon AGI \ \
% \textsuperscript{3}MIT \ \ 
% }}

\begin{document}
\maketitle
\input{sec/6_Appendix}
{
    \small
    \bibliographystyle{ieeenat_fullname}
    \bibliography{main}
}
% WARNING: do not forget to delete the supplementary pages from your submission 

\end{document}
